# Supplementary material for: Convex Sparse Blind Deconvolution
Source: arXiv:2106.07053 source file (2021-06-13)
Supplement: Supplementary file 1 [file appendix_projection_pursuit.tex]

\section{Appendix: Phase Transition Condition for Other Probabilistic Model of Signal}

\subsection{ Phase Transition Condition of Projection Pursuit and Convex Blind Deconvolution for General Probabilistic Model}
Now we state the general phase transition with light assumption. Here we don't need to even assume that $X$ are independent, we just need to know the existence of one sparse element $X_0$.

\begin{theorem}[Projection pursuit to find a sparse element]
\label{thm:sparse_element}
Given a sequence $\{X_t\}_{t\in \integers}$ where one element $X_0$ is a sparse element with $p G + (1-p) \delta_0$ for a symmetric distribution $G$.
Let $\psi^\star$ be the solution of  $P_{u}$:
\[
 \begin{array}{ll}
 \underset{\psi}{\mbox{minimize}}   & \Expect|\psi^T X|\\
\mbox{subject to}  
& u^T \psi =1
\end{array}
\tag{$P_{u}$ }
  \]
then there exists a threshold
$
p^\star
$,
$\psi^\star = e_0$ provided $p<p^\star$,
and  $\psi^\star \neq e_0$ provided $p> p^\star$.

Here $p^\star$ is determined by $G$, the distribution of $\{X_t, t\neq 0\}$ and the direction of $u$:
  \[
  \frac{p^\star}{1-p^\star} =  \inf_{\| \beta\|_2=1, u^T \beta =0} \frac{\Expect[|X_{(0)}^T \beta_{(0)}| \mid X_0 =0]}{\Expect[|G|]\|\beta_{(0)}\|_2} \tan(\angle( \beta, -e_0))
  \]
 where $\beta_{(0)}$ is $\beta$ with the $0-$th entry deleted.

  \end{theorem}

\begin{figure}[!tb]
\centering
\includegraphics[width=.8\textwidth]{./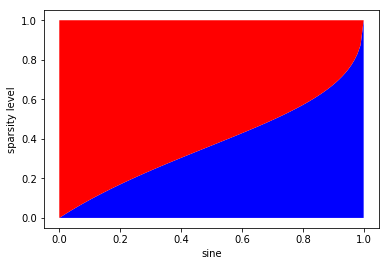}
\caption{The population phase transition diagram of $ \frac{p^\star}{1-p^\star}  = \cot(\angle(u, e_0)) $ for the special case when $X_t$ is independent, $X_0$ is sampled from Bernoulli Gaussian $p N(0,1) +(1-p) \delta_0,$ and the rest $\{X_t, t\neq 0\}$ are sampled from Gaussian $N(0,1)$. The red region is failure, and the blue region is success. }
\label{fig-PT-project}
\end{figure}

\begin{proof}
The phase transition condition proof is based on  calculating the directional derivative.

First, we want to find a threshold $p^\star$ such that for all $p<p^\star$, the directional derivative at $\psi = e_0$ is non-negative along all direction $\beta$ on unit sphere such that $u^T \beta =0$:
	 \[
	 \nabla_{\beta}{\Expect|(e_0+\beta)^T X|}\geq 0
	 \]
Second, we calculate $\nabla_{\beta}{\Expect|(e_0+\beta)^T X|} $ based on whether $X_0$ is zero or not:
	 \[
	 \begin{array}{ll}
	     \nabla_{\beta}{\Expect|(e_0+\beta)^T X|} = p \beta_0 \Expect[|X_{0}| \mid X_0 \neq 0]  + (1-p) \Expect[|X_{(0)}^T \beta_{(0)}| \mid X_0 =0]
	 \end{array}
	\]
It is non-negative in case either $\beta_{0} > 0$, or in case $\beta_0 < 0$ and
	\[
	\frac{p}{1-p} < \frac{\Expect[|X_{(0)}^T \beta_{(0)}| \mid X_0 =0]}{\Expect[|G|]||\beta_0|}
	\]
	for all $\beta \in \{\| \beta\|_2=1, u^T \beta =0\}$.
% 	\item
$p^\star$ is the least upper bound of all $p$ satisfying this inequality. 
Therefore,  
	\[
	\frac{p^\star}{1-p^\star} =  \inf_{\| \beta\|_2=1, u^T \beta =0} \frac{\Expect[|X_{(0)}^T \beta_{(0)}| \mid X_0 =0]}{\Expect[|G|]|\beta_0|} =  \inf_{\| \beta\|_2=1, u^T \beta =0} \frac{\Expect[|X_{(0)}^T \beta_{(0)}| \mid X_0 =0]}{\Expect[|G|]\|\beta_{(0)}\|_2} \tan(\angle( \beta, -e_0))
	\]
\end{proof}

\subsection{Searching for Single Sparse Entry in Gaussian Signal}
\paragraph{Finding one sparse element: Bernoulli Gaussian $X_0$ and Gaussian $\{X_t, t\neq 0\}$}

Now we study the implication of the general phase transition problem in a simplest projection pursuit case, where $X_t$ are independent, $X_0$ is sampled from Bernoulli Gaussian $p N(0,1) +(1-p) \delta_0,$ and the rest $\{X_t, t\neq 0\}$ are sampled from Gaussian $N(0,1)$.

\begin{theorem}
Let $X_t$ be independent, $X_0$ is sampled from Bernoulli Gaussian $p N(0,1) +(1-p) \delta_0,$ the rest $\{X_t, t\neq 0\}$ are sampled from Gaussian $N(0,1)$.
Let $\psi^\star$ be the solution of  $P_{u}$:
\[
 \begin{array}{ll}
 \underset{\psi}{\mbox{minimize}}   & \Expect|\psi^T X|\\
\mbox{subject to}  
& u^T \psi =1
\end{array}
\tag{$P_{u}$ }
  \]
then there exists a threshold
$
p^\star
$,
$\psi^\star = e_0$ provided $p<p^\star$,
and  $\psi^\star \neq e_0$ provided $p> p^\star$.

Here $p^\star$ is determined by the direction of $u$:
  \[
  \frac{p^\star}{1-p^\star} = \inf_{\| \beta\|_2=1, u^T \beta =0}\tan(\angle( \beta, -e_0)) = \cot(\angle(u, e_0))
  \]
  \end{theorem}
\begin{proof}
First, when the rest of $X_t, t\neq 0$ is independent of $X_0$, and IID sampled from $ N(0,1),$
	\[
 \frac{\Expect[|X_{(0)}^T \beta_{(0)}| \mid X_0 =0]}{\|\beta_{(0)}\|_2} = 
\sqrt{\frac{2}{\pi}}
\]
Since  
\[
	 \Expect[|G|] = \sqrt{\frac{2}{\pi}},
	 \]
we have a simple phase transition condition that is completely geometric.
	 \[
  \frac{p^\star}{1-p^\star} = \inf_{\| \beta\|_2=1, u^T \beta =0}\tan(\angle( \beta, -e_0))
  \]
 
Second, we know that there is a geometric structure:
\[
\inf_{\| \beta\|_2=1, u^T \beta =0} \frac{\|\beta_{(0)}\|_2}{|\beta_0|}
= \inf_{\| \beta\|_2=1, u^T \beta =0}\tan(\angle( \beta, -e_0)) = \cot(\angle(u, e_0)),
\]
as indicated by figure~\ref{fig-Angle}. 
When $\beta = P_u^\perp (-e_0)$,
	\[
	\begin{array}{ll}
	\inf_{\| \beta\|_2=1, u^T \beta =0} 
		\tan(\angle( \beta, -e_0)) 
		&=
		\tan(\angle( P_u^\perp (-e_0), -e_0)) \\
		&= \cot(\angle(u, e_0)).
	\end{array}
	\]
	
Therefore, $ \frac{p^\star}{1-p^\star}  = \cot(\angle(u, e_0)) $,

% \begin{figure} 
% \centering
% \includegraphics[width=.8\textwidth]{./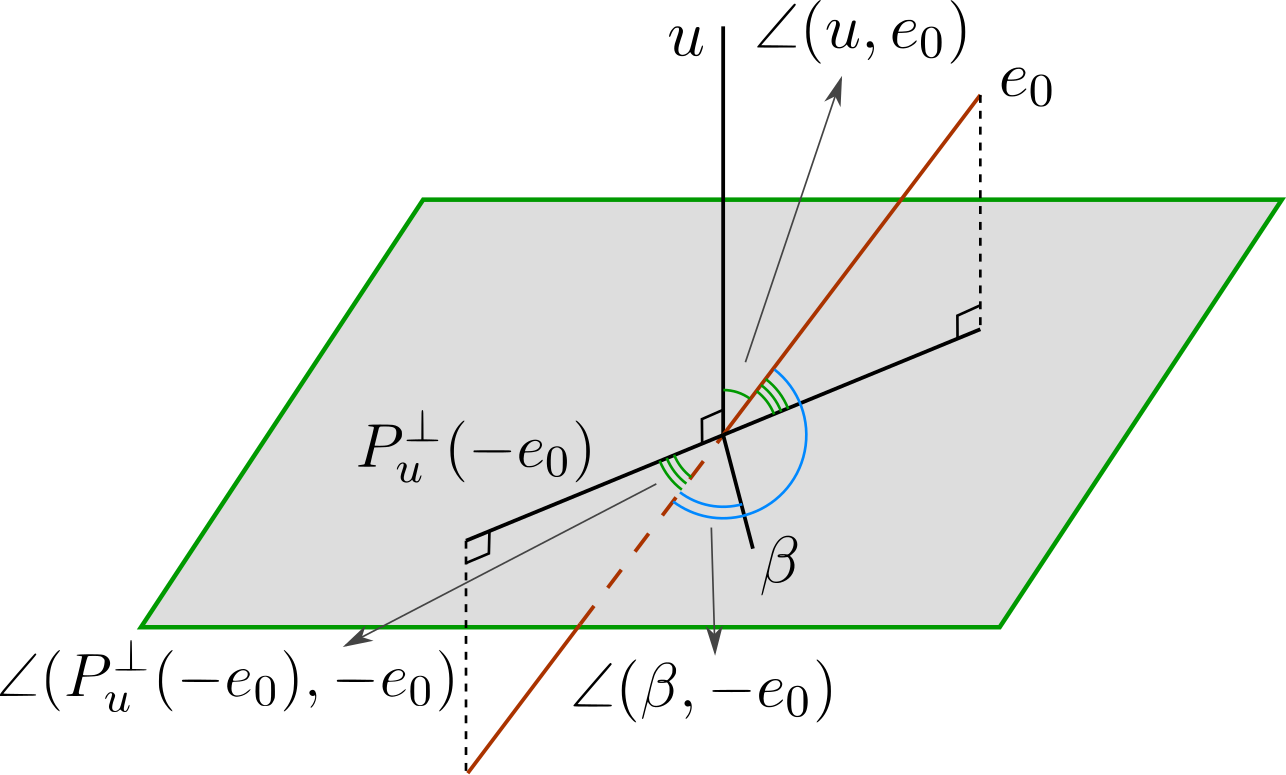}
% \caption{Demonstration of relation between
%   $\angle( \beta, -e_0)$ and ${\angle(u, e_0)}$}
% \label{fig-Angle}
% \end{figure}
\end{proof}
